# Supplementary material for: Path-Invariant Map Networks
Source: arXiv:1812.11647 source file (2019-06-04)
Supplement: Supplementary file 1 [file main_supp.tex]

\documentclass[10pt,twocolumn,letterpaper]{article}

\usepackage{cvpr}
\usepackage{times}
\usepackage{epsfig}
\usepackage{graphicx}
\usepackage{amsmath}
\usepackage{amssymb}
\usepackage{graphicx}
\usepackage{subfig}
\usepackage{caption}
\usepackage{overpic}
\usepackage{wrapfig}
\usepackage{multirow}
\usepackage{wrapfig}

\usepackage{amsthm}
\usepackage{algorithm}
\usepackage{algpseudocode}

\makeatletter
\@namedef{ver@everyshi.sty}{}
\makeatother
\usepackage{tikz}
\usetikzlibrary{arrows, snakes, backgrounds, positioning}
\usepackage{tikzscale}

% math equations that are widely used

\def \saliency {\textup{\saliency}}

\def \path {\textup{path}}

\makeatother

\theoremstyle{plain}

 \theoremstyle{definition}
\numberwithin{theorem}{section}
\numberwithin{lem}{section}

\theoremstyle{remark}

 %\newcommand{\para}[1]{\noindent{\bf #1}\hspace{1em}}
%\newcommand{\set}[1]{{\textstyle{\mathcal #1}}}

% Include other packages here, before hyperref.

% If you comment hyperref and then uncomment it, you should delete
% egpaper.aux before re-running latex.  (Or just hit 'q' on the first latex
% run, let it finish, and you should be clear).
\usepackage[pagebackref=true,breaklinks=true,letterpaper=true,colorlinks,bookmarks=false]{hyperref}

% \cvprfinalcopy % *** Uncomment this line for the final submission

 % *** Enter the CVPR Paper ID here

% Pages are numbered in submission mode, and unnumbered in camera-ready
\ifcvprfinal\pagestyle{empty}\fi
\begin{document}

%%%%%%%%% TITLE
\title{Path-Invariant Map Networks Supplemental Material}

\author{Zaiwei Zhang\\
Department of Computer Science\\
The University of Texas at Austin\\
Austin, TX 78712, USA \\
{\tt\small zaiweizhang@utexas.edu}
% For a paper whose authors are all at the same institution,
% omit the following lines up until the closing ``}''.
% Additional authors and addresses can be added with ``\and'',
% just like the second author.
% To save space, use either the email address or home page, not both
\and
Zhenxiao Liang\\
Department of Computer Science\\
The University of Texas at Austin\\
Austin, TX 78712, USA \\
{\tt\small liangzx@cs.utexas.edu}
\and
Lemeng Wu\\
Department of Computer Science\\
The University of Texas at Austin\\
Austin, TX 78712, USA \\
{\tt\small lmwu@cs.utexas.edu}
\and
Xiaowei Zhou\\
Zhejiang University\\
Hangzhou, China, 310058\\
{\tt\small xzhou@cad.zju.edu.cn}
\and
Qixing Huang\\
Department of Computer Science\\
The University of Texas at Austin\\
Austin, TX 78712, USA \\
{\tt\small huangqx@cs.utexas.edu}
}

\maketitle

\input{app_01_overview.tex}
\input{app_02_proof.tex}
\input{app_04_dense_map.tex}
\input{app_05_3D_representation.tex}
\input{app_03_shape_matching.tex}

{\small
\bibliographystyle{ieee}
\bibliography{cycle}
}
\newpage
\appendix

\end{document}
